# Supplementary material for: Rhythmomimetic drug delivery: modeling, analysis and numerical simulation
Source: arXiv:1512.05758 source file (2016-04-05)
Supplement: Supplementary file 1 [file supplement.pdf]

**S. Supplementary Material.** This section involves two parts, one includes parameters of the model used in experiments as well as simulations. The second one contains background materials on competitive dynamical systems, supplementing section 8 of the article.

**S.1. Model scaling and the governing system.** These tables provide detail on the experimental range of parameters of the problem that give oscillatory behaviour.

TABLE S.1
*Fields of the model*

| L | $\phi$ | x | y | z | $\lambda$ | f |
|---|---|---|---|---|---|---|
| Membrane Length | polymer volume fraction | $C_{\mathrm{H}}$ | $C_{\mathrm{AH}}$ | $C_{\mathrm{H}}^{II}$ | Donnan ratio | Ionization fraction of carboxyls |

TABLE S.2
*Parameters of the device*

| $L_0$ | $A$ | $V$ | h | $C_{\mathrm{NaCl}}$ | $C_{\mathrm{G}}$ |
|---|---|---|---|---|---|
| Ref.memb.length | Cross-sect memb.area | Chamber Vol. | $H^+$ conc. cell I | Salt conc. | Glucose conc. |
| 250 $\mu$m | 314 cm$^2$ | 75ml | $10^{-7}$ M | $1.55 \times 10^{-1}$M | $50 \times 10^{-3} M$ |

TABLE S.3
*Hydrogel Parameters*

| $\chi_1$ | $\chi_2$ | $K_{\mathrm{A}}$ | $\phi_0$ | $\sigma_0$ | $\rho_0$ |
|---|---|---|---|---|---|
| Flory-Huggins par. | Flory-Huggins par. | Dissoc.const.carboxyl | Pol.ref.vol.frac. | Ref.conc.carboxyl | Pol.ref crosslink dens. |
| 0.43 | 0.6 | $10^{-4.5}$ M | 0.3 | 0.28 M | 0.014 M |

An additional parameter of the system is the *molar volume* of water, $v_{\mathrm{w}} = 18$ ml/mol.

**S.2. Competitive systems and three-dimensional limit cycles.**

**S.2.1. Definitions.**

1. A dynamical system $\varphi_t$ is *monotone* in $\mathbb{R}^n$ provided $\varphi_t(\mathbf{y}) \leq \varphi_t(\mathbf{x})$ whenever $\mathbf{y} \leq \mathbf{x}$. This is a formal expression of the corresponding inequalities satisfied by each component.
2. We say that $\mathcal{D}$ is p-*convex* if $t\mathbf{x} + (1-t)\mathbf{y} \in \mathcal{D}$ for all $t \in [0,1]$ whenever $\mathbf{x}, \mathbf{y} \in \mathcal{D}$ and $\mathbf{x} \leq \mathbf{y}$. Note that if $\mathcal{D}$ is convex is also p-convex.

In order to make precise the concept of monotonic dynamical system, we define the nonnegative cone $\mathbf{R}^n_+$ in $\mathbf{R}^n$ as the set of all n-tuples with nonnegative coordinates. With this, the concept of partial order naturally arises as $\mathbf{y} \leq \mathbf{x}$ if $\mathbf{x} - \mathbf{y} \in \mathbf{R}^n_+$. The definitions of strict order can be stated in the analogous manner.

**The Kamke Condition.** The vector field $\boldsymbol{f}$ is said to be of *type K* in $\mathcal{D}$ if $f_i(\mathbf{a}) \leq f_i(\mathbf{b})$ whenever $\mathbf{a} \leq \mathbf{b}$ and $a_i = b_i$, for some $1 \leq i \leq n$.

The following result, stated as a remark in [**?**], gives criteria to characterize type K systems in terms of the sign structure of the Jacobian matrix of the system. The proof is a direct consequence of the fundamental theorem of calculus.

LEMMA S.1. *If $\mathcal{D}$ is a p-convex subset of $\mathbf{R}^n$ and*

$$\frac{\partial f_i}{\partial x_j}(\mathbf{x}) \geq 0, \quad i \neq j, \ \mathbf{x} \in \mathcal{D} \tag{S.1}$$

*holds, then $\boldsymbol{f}$ is of type K in $\mathcal{D}$.*

**Definitions.** The system $\dot{\mathbf{x}} = \boldsymbol{f}(\mathbf{x})$ is *cooperative* if (S.1) holds on the p-convex domain $\mathcal{I}$. A dynamical system is called *competitive* if

$$\frac{\partial f_i}{\partial x_j}(\mathbf{x}) \leq 0, \quad i \neq j, \ \mathbf{x} \in \mathcal{I}. \tag{S.2}$$

A competitive system becomes cooperative by time reversal, and vice-versa.

TABLE S.4
*Rate Parameters*

| Permeability coeff. $H^+$ | Permeability coeff. water | Sieving effect of pol. | Marble reaction rate | Glucose reaction rate* |
|---|---|---|---|---|
| $K_{\mathrm{H}}$ | $K_w$ | $\beta$ | $k_{\mathrm{mar}}$ | $K_G^0$ |
| $2.5 * 10^{-3}$ cm/sec | $1.5 * 10^{-2}$ cm/sec | 13.5 cm/sec | $50 * 10^{-3}$ cm/sec | $5 * 10^{-4}$cm/sec |

Cooperative and competitive systems generate monotone dynamical systems. In particular, a competitive system has the property that the time reverse flow is monotone: if $\mathbf{x} \leq \mathbf{y}$ and $t < 0$, then $\varphi_t(\mathbf{x}) \leq \varphi_t(\mathbf{y})$. This implies that the forward flow of a competitive dynamical system preserves the property of two points being unrelated. ($\mathbf{x}$ and $\mathbf{y}$ are called *unrelated* if neither $\mathbf{x} \leq \mathbf{y}$ nor $\mathbf{y} \leq \mathbf{x}$ holds.) Indeed, if $\varphi_t(\mathbf{x})$ and $\varphi_t(\mathbf{y})$ were related at some $t > 0$, then $\mathbf{x}$ and $\mathbf{y}$ would be related by time reversal.

**S.2.2. Competitive dynamical systems in alternate cones.** Many systems of interest are competitive in a more general sense as in the case of the problem analysed in this article. In fact, the theory of competitive systems can be extended to the case of general cones $\mathcal{K} \subset \mathbf{R}^n$, in particular, those consisting of intersections of half-spaces. The order relations $\mathbf{x} \leq \mathbf{y}$, which can expressed as $< \mathbf{y} - \mathbf{x}, \mathbf{e}_i >$, where $< \cdot, \cdot >$ denotes the Euclidean inner product, and $\mathbf{e}_i$ a vector of the canonical basis, can be generalized to requiring $g(\mathbf{y} - \mathbf{x}) \geq 0$, for some $g \in \mathcal{K}^*$, the *dual* space of $\mathcal{K}$.

For the system to be competitive with respect to a general cone, it must, first, satisfy the following two properties:

DEFINITION S.2. *An $n \times n$ matrix is sign-stable in $\mathcal{D}$ if for each $i \neq j$, either $\frac{\partial f_i}{\partial x_j} \geq 0$ for all $\mathbf{x} \in \mathcal{D}$, or $\frac{\partial f_i}{\partial x_j} \leq 0$ for all $\mathbf{x} \in \mathcal{D}$. The matrix is called sign-symmetric if $\frac{\partial f_i}{\partial x_j}(\mathbf{x})\frac{\partial f_j}{\partial x_i}(\mathbf{y}) \geq 0$ for all $i \neq j$, and all $\mathbf{x}, \mathbf{y} \in \mathcal{D}$.*
The sign structure of the system (6.6)-(5.9) is symbolically represented by the diagram:

$$\begin{vmatrix} * & + & 0 \\ + & * & + \\ - & + & * \end{vmatrix}. \tag{S.3}$$

To show that the system is competitive, we further explore the monotonicity relations in the system. This issue is related with the identification of the cone structure of the problem. For this, we apply the algorithm that derives from ([34], Proposition 5.1, page 48). Let us assign digits $s_{ij} \in \{0, 1\}$, $1 \leq i < j \leq 3$ as follows:

$$s_{ij} = 1, \text{ if } \frac{\partial f_i}{\partial x_j} + \frac{\partial f_j}{\partial x_i} > 0 \quad \text{and} \quad s_{ij} = 0, \text{ if } \frac{\partial f_i}{\partial x_j} + \frac{\partial f_j}{\partial x_i} < 0, \tag{S.4}$$

for some $x \in \mathcal{D}$. Now, we consider the system of 3 linear equations in the unknowns $m_{ij} \in \{0, 1\}$, $1 \leq i < j \leq 3\}$, such that

$$m_i + m_j = s_{ij} \pmod 2. \tag{S.5}$$

If these equations have a solution, then the system is competitive with respect to the cone $\mathcal{K}_m$, $m = (m_1, m_2, m_3)$. It is easy to check that for the matrix with sign structure (**??**) $s_{12} = 1 = s_{23}$ and $s_{13} = 0$. For the Jacobian matrix of the problem, the system (S.5) admits the solution $m_1 = m_3 = 1$ and $m_2 = 0$. From these relations, existence of a competitive cone for the system follows.
